# Supplementary material for: Deep COVID-19 Forecasting for Multiple States with Data Augmentation
Source: arXiv:2302.01155 source file (2023-02-02)
Supplement: Supplementary file 1 [file x1_appendix.tex]

\documentclass[main.tex]{subfiles}
\begin{document}
\appendix

%%%%%%%%%%%%%%%%%%%%%%%%%%%%%%%%%%%%%%%%%%%%%%%%%%
\section{Appendix}
\label{sec:appendix_a}
%%%%%%%%%%%%%%%%%%%%%%%%%%%%%%%%%%%%%%%%%%%%%%%%%%

\end{document}
